# Supplementary material for: Queue Length Simulation for Signalized Arterial Networks and Steady State Computation under Fixed Time Control
Source: arXiv:1705.07493 source file (2017-09-11)
Supplement: Supplementary file 1 [file appendix-existence-v2.tex]

\subsection{Proof of Proposition~\ref{prop:solution-properties}}
\label{sec:existence}
%It is sufficient to show the existence and uniqueness of solution to \eqref{z-linprog}; \eqref{eq:outflow-expr-compact} follows from \eqref{z-linprog} trivially.
We first note that, for a given $t \geq 0$, $z(t-\delta_{ji})$ is given for link pairs $(j,i)$ for which $\delta_{ji}>0$. For every $i \in \mc E$, let 
\begin{equation}
\label{eq:E-i-def}
\mc E_i:=\setdef{j \in \mc E}{R_{ji} > 0 \quad \& \quad \delta_{ji} = 0}
\end{equation}
 be the set of links incoming to $i$ with strictly positive travel times. For brevity in presentation, let $\tilde{\lambda}_i(t):=\lambda_i(t)+\sum_{j \in \mc E \setminus \mc E_i} R_{ji} z_j(t-\delta_{ji})$, $i \in \mc E$. Therefore, \eqref{z-linprog} can be rewritten as:
 \begin{equation}
\begin{aligned}
& \underset{z \in \real^{\mc E}}{\text{maximize}} \qquad \eta^{T} z \\
%& \alpha^{T}z \\
& \text{subject to} \qquad \qquad  z_i \leq c_i(t), \qquad i \in \mc E   \\
%&  z_i \leq y_i, \; \qquad \forall i \in  {\mc E} \\
&  \qquad \qquad \qquad  z_i \leq \tilde{\lambda}_i(t) + \sum_{j \in \mc E_i} R_{ji} z_j, \qquad i \in \mc E^{\text{temp}}_0  \\
\end{aligned}
\label{z-linprog-new}
\end{equation}

The feasible set for \eqref{z-linprog-new} is non-empty ($z=0$ is always feasible) and compact. Therefore, there exists at least one solution, say $\hat{z}$, to \eqref{z-linprog-new}. 
For every $i \in \mc E$, $\hat{z}_i$ satisfies at least one of the two inequalities in \eqref{z-linprog-new} with equality. If this is not the case, say for $\hat{z}_i$, one can increase it until at least one of the two inequalities is satisfied. The only other second set of inequalities in \eqref{z-linprog-new} that such a change affects are the ones corresponding to links in $\mc E_i$. Increasing $\hat{z}_i$ leads to increase in the right hand side of these inequalities, thereby maintaining feasibility. 
On the other hand, increasing $\hat{z}_i$ also strictly increases the objective function thereby contradicting that $\hat{z}$ is optimal. Let \ksmargin{the proof for uniqueness can possibly be reduced}
\begin{equation}
\label{eq:K1-K2-def}
\mc K_1:=\setdef{i \in \mc E}{\hat{z}_i=c_i(t)}, \quad \mc K_2:=\setdef{i \in \mc E}{\hat{z}_i=\tilde{\lambda}_i(t) + \sum_{j \in \mc E_i} R_{ji} \hat{z}_j}
\end{equation} 
be a covering of $\mc E$.
In particular, note that $\mc K_1^c := \mc E \setminus \mc K_1 \subseteq \mc K_2$. 
%\kscomment{Lemma~\ref{lem:solution-properties} implies that $\mc E = \mc I \cup \mc J$.}
In order to show uniqueness, following, e.g., \cite[Theorem 2]{Mangasarian:79}, it is sufficient to show that there is no $z \neq 0$ satisfying the following:
\begin{align}
\label{eq:uniqueness}
\begin{split}
\eta^T z & \geq 0; \qquad z_i \leq 0, \quad \forall \, i \in \mc K_1; \\ z_i & \leq \sum_{j \in \mc E_i} R_{ji} z_j, \quad \forall \, i \in \mc K_2 
\end{split}
\end{align}
By contradiction, assume that there exists $z$ satisfying \eqref{eq:uniqueness}. In particular, this implies that $\bar{\mc E}:=\setdef{i \in \mc E}{z_i > 0} \subseteq \mc K_1^c \subseteq \mc K_2$ is not empty. Therefore, the last constraint in \eqref{eq:uniqueness} implies that
\begin{equation}
\label{eq:uniqueness-alternate}
z_i \leq \sum_{j \in \bar{\mc E} \cap \mc E_i} R_{ji} z_j, \qquad \forall \, i \in \mc K_2 \supseteq \bar{\mc E}
\end{equation}
which in turn implies that 
\begin{equation}
\label{eq:uniqueness-implication}
\setdef{j \in \bar{\mc E} \cap \mc E_i}{\tau_j = \sigma_i, \, R_{ji} > 0} \neq \emptyset, \qquad \forall \, i \in \bar{\mc E} 
\end{equation}
%Let $\bar{\mc G}:=(\mc V, \bar{\mc E})$. 

\ksmargin{show $v$, $j_2$, $j_3$ in Fig~\ref{fig:uniqueness}}
\begin{figure}[htb!]
\begin{center}				
\includegraphics[width=1.52in,angle=270]{../CDC2017/fig/uniqueness-illustration.pdf} 
\end{center}
\caption{Illustration of construction to prove uniqueness of solution to \eqref{z-linprog}.}
\label{fig:uniqueness}
\end{figure}

Pick an arbitrary node $v \in \mc V$ such that $\bar{\mc E}_v^- \cap \mc E_i \neq \emptyset$. Let $j_1 = \argmax_{i \in \bar{\mc E}_v^- \cap \mc E_i} z_i$ (ties are broken arbitrarily). Following \eqref{eq:uniqueness-implication}, let $j_2:=\argmax_{i \in \bar{\mc E}_{\sigma(j_1)}^-\cap \mc E_{j_1}} \, z_i$, with ties broken arbitrarily. The definition of $j_2$, along with \eqref{eq:uniqueness-implication} implies that $z_{j_1} \leq z_{j_2}$.
%
%and the fact that $R_{ij} < 1$ for all $i, j \in \mc E$, implies that $b_{j_1} < b_{j_2}$. 
One can similarly find $j_3$ such that $z_{j_1} \leq z_{j_2} \leq z_{j_3}$. Following \eqref{eq:uniqueness-implication}, this process can be repeated at most $m \leq |\mc V|$ times, when 
\begin{equation}
\label{eq:b-inequalities}
0< z_{j_1} \leq \ldots \leq z_{j_m}
\end{equation}
and $\sigma_{j_m}=\tau_{j_k}$ for some $k \in \until{m-1}$: see Figure~\ref{fig:uniqueness} for illustration. The definition of $j_k$ along with \eqref{eq:uniqueness-alternate} then implies that $z_{j_m} \leq z_{j_k}$, which, in light of \eqref{eq:b-inequalities}, can be true only if $z_{j_k} = \ldots z_{j_m}$. However, this implies that $R_{j_\ell j_{\ell-1}}=1$ for all $\ell \in \{k+1, \ldots,m\}$ and $R_{j_k j_m}=1$, i.e., the sub-network consisting of links $j_k, \ldots, j_m$ is a connected component. However, the fact that $R_{j_\ell j_{\ell-1}}=1$ for all $\ell \in \{k+1, \ldots,m\}$ and $R_{j_k j_m}=1$ then violates Assumption~\ref{ass:routing-matrix} (a).  
%In this case, \eqref{eq:uniqueness} holds true independently for this sub-network. However, this leads to a contradiction due to \eqref{eq:b-inequalities}. 
Therefore, $\bar{\mc E}=\emptyset$, and hence there does not exist $z \neq 0$ satisfying \eqref{eq:uniqueness}. Hence, $\hat{z}$ is the unique solution for a given $\eta \in \real_{>0}^{\mc E}$.

In order to prove that the optimal solution to \eqref{z-linprog-new} is independent of $\eta$, first note that if $z$ and $\tilde{z}$ satisfy the constraints in \eqref{z-linprog-new}, then so does $z^{\text{max}}$ defined by $z_i^{\text{max}}=\max\{z_i,\tilde{z}_i\}$ for all $i \in \mc E$. This is because $z \leq c(t)$ and $\tilde{z} \leq c(t)$ implies that $z^{\text{max}} \leq c(t)$, and therefore the first inequality in \eqref{z-linprog-new} is trivially satisfied by $z^{\text{max}}$. With respect to the second inequality, fix some $i \in \mc E_0^{\text{temp}}$, and let $z_i^{\text{max}}=z_i$ (without loss of generality). 
Then, 
$
z_i^{\text{max}}=z_i \leq \tilde{\lambda}_i + \sum_{j \in \mc E_i: \, z_j^{\text{max}}=z_j} R_{ji} z_j + \sum_{j \in \mc E_i: \, z_j^{\text{max}}=\tilde{z}_j} R_{ji} z_j \leq \tilde{\lambda}_i +\sum_{j \in \mc E_i: \, z_j^{\text{max}}=z_j} R_{ji} z^{\text{max}}_j + \sum_{j \in \mc E_i: \, z_j^{\text{max}}=\tilde{z}_j} R_{ji} z^{\text{max}}_j = \tilde{\lambda}_i + \sum_{j \in \mc E_i} R_{ji}  z_j^{\text{max}}$, 
where the first inequality follows from \eqref{z-linprog-new} and the second one follows from the definition of $z^{\text{max}}$.

Therefore, if $z \neq \tilde{z}$, then $z^{\text{max}} \neq z \neq \tilde{z}$ and hence $z$ and $\tilde{z}$ can not be the optimal solution to \eqref{z-linprog-new} for any $\eta >0$. In particular, if $z$ and $\tilde{z}$ are the unique optimal solutions corresponding to $\eta \in \real_{>0}^{\mc E}$ and $\tilde{\eta} \in \real_{>0}^{\mc E}$ and $z \neq \tilde{z}$, then we get a contradiction that $z$ and $\tilde{z}$ can not be optimal solutions corresponding to either $\eta$ or $\tilde{\eta}$. 
