# Supplementary material for: Queue Length Simulation for Signalized Arterial Networks and Steady State Computation under Fixed Time Control
Source: arXiv:1705.07493 source file (2017-09-11)
Supplement: Supplementary file 2 [file appendix-jump.tex]

%\begin{lemma}
%For any $\lambda \in \real_+^{\mc E}$ and $c \in \real_+^{\mc E}$, the iterative procedure terminates in finite steps.
%\end{lemma}
%\begin{proof}
%Let the sequence of $\mc E_0(x)$ generated by the iterative procedure described above be denoted as $\mc E_1, \mc E_2, \ldots$. We now show that this sequence is strictly monotonically decreasing and hence, due to finite number of values that the sequence can take, the procedure terminates in finite iterations. 
%\end{proof}
