# Supplementary material for: Queue Length Simulation for Signalized Arterial Networks and Steady State Computation under Fixed Time Control
Source: arXiv:1705.07493 source file (2017-09-11)
Supplement: Supplementary file 4 [file appendix-existence-dynamics-very-old.tex]

\subsection{Proof of Proposition~\ref{prop:existence-traffic-dynamics-solution}}
\ksmargin{add more details here}
\kscomment{The proof for the case when $\underline{\delta}>0$ is relatively straightforward.} Indeed, in this case:
\begin{equation*}
\label{eq:z-expr-positive-travel-time}
z_i(x,t)= \begin{cases} c_i(t) & i \in \mc E \setminus \mc E_0(x) \\
\lambda_i(t)+\sum_j R_{ji} z_j(t-\delta_{ji}) & i \in \mc E_0(x)
\end{cases}
\end{equation*}

The proof for the case when $\lambda(t)$ and $c(t)$ are piecewise constant follows once we establish that the jumps in $\mc E_0(x(t))$ 
are finite over a given time interval under the dynamics in \eqref{eq:flow-dynamics}. This is because in between jumps, Algorithm~\ref{alg:z-computation} implies that $z(x,t)$ is also piecewise constant, and hence the solution to \eqref{eq:flow-dynamics} exists. Indeed, it is sufficient to show that the number of jumps are finite during any interval over which $\lambda(t)$ and $c(t)$ is constant. Therefore, for the rest of the section, we establish finiteness of the number of jumps when $\lambda(t) \equiv \lambda$ and $c(t) \equiv c$, starting from any initial condition $x_0 \in \real_+^{\mc E}$. 

\begin{proposition}
\label{prop:monotonic-increase-zero-set}
Let $\lambda(t) \equiv \lambda \geq 0$ and $c(t) \equiv c \geq 0$. Then, under the dynamics in \eqref{eq:flow-dynamics}, for any $x_0 \in \real_+^{\mc E}$, $\mc E_0(x(t_1)) \subseteq \mc E_0(x(t_2))$ if $t_1 < t_2$.
\end{proposition} \ksmargin{need to add a lot more details here}

Since the total number of values that $\mc E_0(x)$ can take is $2^{\mc E}$, Proposition~\ref{prop:monotonic-increase-zero-set} implies that there are at most $2^{\mc E}$ switches in $\mc E_0(x)$ when the external inflows and capacity functions are constant. The proof of Proposition~\ref{prop:monotonic-increase-zero-set} relies on a couple of technical lemmas which follow next. 
%if $\lambda_i(t)$ and $c_i(t)$ are constant for all $i \in \mc E$ over that time interval. The result can then be extended straightforwardly to any time interval over which Assumption~\ref{ass:piecewise-constant} is satisfied. 
\ksmargin{should we define connected components ?}
The first lemma shows that \eqref{z-linprog} can be decomposed into \kscomment{connected components} of $\mc E_0^{\text{temp}}$. 

\ksmargin{Lemma~\ref{lem:linprog-decomposition} needs to be adapted for the case when $\delta_{ji} > 0$.}
\begin{lemma}
\label{lem:linprog-decomposition}
Consider the linear program in \eqref{z-linprog} for given $t \geq 0$, $\mc E_0^{\text{temp}}$, $\lambda(t)$, $c(t)$ and $\{z(s): \, s \in [t-\bar{\delta},t)\}$. 
Let the connected components of $\mc E_0^{\text{temp}}$ be $\mc E_0^1, \ldots, \mc E_0^r$, and let
%For any $x \in \real_+^{\mc E}$, let $\tilde{\mc E}^{(1)}(x), \ldots, \tilde{\mc E}^{(r)}(x)$ be the connected components of $\tilde{\mc E}(x)$. Let 
the corresponding components of $z^{\text{temp}}$ and $\eta$ be $z^{1}, \ldots, z^{r}$ and $\eta^{1}, \ldots, \eta^{r}$, respectively. 
Then, the solution to \eqref{z-linprog} is $z_i^{\text{temp}}=c_i(t)$ for $i \in \mc E \setminus \mc E_0^{\text{temp}}$, and, $z^{k}$ for $k \in \until{r}$ is given by the unique solution to the following linear program:
\begin{equation*}
\begin{aligned}
& \underset{z \in \real^{\mc E_0^{k}}}{\text{maximize}} \qquad {\eta^{k}}^{T} z \\
%& \alpha^{T}z \\
& \text{subject to} \qquad \qquad  z_i \leq c_i(t), \qquad i \in \mc E_0^k   \\
%&  z_i \leq y_i, \; \qquad \forall i \in  {\mc E} \\
&  \qquad \qquad \qquad  z_i \leq \lambda_i(t) + \sum_{j \in \mc E: \, \delta_{ji}>0} R_{ji} z_j(x,t-\delta_{ji}) +
\sum_{j \in \mc E \setminus \mc E_0^k: \, \delta_{ji} = 0} R_{ji} c_j(t) + \sum_{j \in \mc E_0^k: \, \delta_{ji} = 0} R_{ji} z_j, \qquad i \in \mc E_0^k  \\
\end{aligned}
\label{z-linprog-component}
\end{equation*}
\end{lemma}
\begin{proof}
\kscomment{(brief proof to be written)}
\end{proof}
%\begin{assumption}
%\label{ass:piecewise-constant}
%The external inflow $\lambda_i(t)$ and capacity functions $c_i(t)$ are piecewise constant for all $i \in \mc E$.
%\end{assumption}

\ksmargin{changed notation from $\tilde{\mc E}$ to $\mc E_0$}
%The main challenge in showing the existence is in characterizing \emph{jumps} in the set \kscomment{$\mc E_0(x)$} defined in \eqref{eq:E-tilde-def} during the evolution governed by \eqref{eq:flow-dynamics}-\eqref{z-linprog}. 
%We say that a jump occurs at time instant $t$ if $\mc E_0(x(t)) \neq \mc E_0(x(t^-))$. 
 
%For given $x \in \real_+^{\mc E}$, let $\hat{\mc E}(x):=\setdef{i \in \mc E}{x_i=0 \, \, \& \, \, c_i > \lambda_i + \sum_{j} R_{ji} \kscomment{z_j(x)}}$. 
%Similarly, let $\hat{\mc G}(x) := (\hat{\mc V}(x), \hat{\mc E}(x))$, where $\hat{\mc V}(x):= \cup_{i \in \hat{\mc E}(x)} \{\sigma_i, \tau_i\}$ is the set of end nodes of links in $\hat{\mc E}(x)$. 

The next lemma establishes useful monotonicity properties, where we recall the definition of $\mc I(x)$ from \eqref{eq:I-def}.

\ksmargin{add more details here and extend the proof to $\delta_{ji}>0$ case}
\begin{lemma}
\label{lem:outflow-monotonicity}
Let $\lambda(t) \equiv \lambda \geq 0$ and $c(t) \equiv c \geq 0$. For any $x, \hat{x} \in \real_+^{\mc E}$:
\begin{enumerate}
\item[(a)] if $\mc E_0(x) \subseteq \mc E_0(\hat{x})$, then $z(x) \geq z(\hat{x})$; and
\item[(b)] if $\mc I(x) \subseteq \mc I(\hat{x})$, then $\mc E_0(x) \supseteq \mc E_0(\hat{x})$
\end{enumerate}
%
%Fix $\lambda_i \geq 0$ and $c_i \geq 0$ for all $i \in \mc E$. If $\mc E_0(x) \subset \mc E_0(\hat{x})$ for some $x, \hat{x} \in \real_+^{\mc E}$, then the solution to \eqref{z-linprog} satisfies $z_i(x) \geq z_i(\hat{x})$ for all $i \in \mc E$. 
\end{lemma}
\begin{proof}
It suffices to prove (a) for a connected component in $\mc E_0(\hat{x})$, say $\tilde{\mc E}(\hat{x})$. 
%Let $\tilde{\mc E}(x)$ denote the corresponding set of links in $\mc E_0(x)$. 
It is further sufficient to consider the non-trivial case when there exists at least one $i \in \tilde{\mc E}(\hat{x})$ such that $x_i>0$. Indeed, for all such $i$,  and for all $i \in \mc E \setminus \mc E_0(\hat{x})$, $z_i(x)=c_i \geq z_i(\hat{x})$. Therefore, \kscomment{taking into account Lemma~\ref{lem:linprog-decomposition}}, the  constraint on $z_i$ for $i \in \tilde{\mc E}(\hat{x}) \setminus \tilde{\mc E}(x)$ is relaxed at $x$ than at $\hat{x}$, which implies (a). 
%\end{proof}
%
%\begin{lemma}
%\label{lem:set-monotonicity}
%Consider the procedure described above to obtain $\mc E_0(x)$. For a given $\lambda_i$ and $c_i$, $i \in \mc E$, if $\mc I(\hat{x}) \supseteq \mc I(x)$, then $\mc E_0(x) \supseteq \mc E_0(\hat{x})$.
%\end{lemma} 
%\begin{proof}

Let the $\mc E_0^{\text{temp}}$ sets computed while executing iterations of Algorithm~\ref{alg:z-computation} for $\mc E_0(x)$ and $\mc E_0(\hat{x})$ be denoted by $\{ \mc E_0^{(1)}(x), \mc E_0^{(2)}(x), \ldots\}$ and $\{\mc E_0^{(1)}(\hat{x}), \mc E_0^{(2)}(\hat{x}), \ldots\}$ respectively. Similarly, let $\{z^{(1)}(x), z^{(2)}(x), \ldots\}$ and $\{z^{(1)}(\hat{x}), z^{(2)}(\hat{x}), \ldots\}$ denote the $z^{\text{temp}}$ computed during the corresponding iterations. Since $\mc I(\hat{x}) \supseteq \mc I(x)$, (a) implies that $z^{(1)}(x) \leq z^{(1)}(\hat{x})$, which in turn \kscomment{straightforwardly} implies that $\mc E^{(1)}(x) \supseteq \mc E^{(1)}(\hat{x})$. Repeated application of this argument for every iteration then gives (b).
\end{proof}

The proof of Proposition~\ref{prop:monotonic-increase-zero-set} is now almost immediate. We show that $\mc E_0(x(s^-)) \subseteq \mc E_0(x(s))$ for all $s \in (t_1,t_2]$. This is true by definition if there is no jump at $s$. If there is a jump at $s$, then it is easy to see that $\mc I(x(s^-)) \subsetneq \mc I(x(s))$. Lemma~\ref{lem:outflow-monotonicity} then gives the proposition.
%
%
%The result is trivially true if there is no jump in $\mc E_0(x(t))$ for $t \in (t_1,t_2]$. Therefore, without loss of generality, assume that there is exactly one jump during this interval, say at $s \in (t_1,t_2]$. We need to show that $\mc E_0(x(s^-)) \subsetneq \mc E_0(x(s))$. Since $\mc E_0(x(s^-)) \neq \mc E_0(x(s))$ ($s$ being a time instant of jump), assume by contradiction that $\mc E_0(x(s^-)) \supsetneq \mc E_0(x(s))$. However, since $\mc E_0^{(0)}(x(s^-)) \subsetneq \mc E_0^{(0)}(x(s))$, Lemma~\ref{lem:set-monotonicity} implies that $\mc E_0(x(s^-)) \subseteq \mc E_0(x(s))$ leading to a contradiction. 
