# Supplementary material for: Queue Length Simulation for Signalized Arterial Networks and Steady State Computation under Fixed Time Control
Source: arXiv:1705.07493 source file (2017-09-11)
Supplement: Supplementary file 6 [file appendix-existence-very-old.tex]

\subsection{Proof of Proposition~\ref{prop:solution-properties}}
\label{sec:existence}
\ksmargin{the proof needs revision not the least to extend it to $\bar{\delta}>0$}
It is sufficient to show the existence and uniqueness of solution to \eqref{z-linprog}; \eqref{eq:outflow-expr-compact} follows from \eqref{z-linprog} trivially.

The feasible set for \eqref{z-linprog} is non-empty ($z=0$ is always feasible) and compact for every $x \in \real_+^{\mc E}$. Therefore, there exists at least one solution, say $\bar{z}$, to \eqref{z-linprog}. 
%\kscomment{Lemma~\ref{lem:solution-properties} implies that $\mc E = \mc I \cup \mc J$.}
In order to show uniqueness, following, e.g., \cite[Theorem 2]{Mangasarian:79}, it is sufficient to show that there is no $z \neq 0$ satisfying the following:
\begin{align}
\label{eq:uniqueness}
\begin{split}
\eta^T z & \geq 0; \qquad z_i \leq 0, \quad \forall \, i \in \mc I; \\ z_i & \leq \sum_{j \in \mc E} R_{ji} z_j, \quad \forall \, i \in \mc J 
\end{split}
\end{align}
where $\mc I:=\setdef{i}{\bar{z}_i=c_i(t)}$ and $\mc J:=\setdef{i}{\bar{z}_i=\lambda_i + \sum_{j \in \mc E} R_{ji} \bar{z}_j}$. By contradiction, assume that such a $z$ exists. Combining this with the fact that $z \neq 0$ and $\eta^T z \geq 0$ from \eqref{eq:uniqueness}, we get that $\bar{\mc E}:=\setdef{i \in \mc E}{z_i > 0}$ is not empty. Therefore, the last constraint in \eqref{eq:uniqueness} implies that
\begin{equation}
\label{eq:uniqueness-alternate}
z_i \leq \sum_{j \in \bar{\mc E}} R_{ji} z_j, \qquad \forall \, i \in \mc J
\end{equation}
\eqref{eq:uniqueness-alternate} implies that, 
\begin{equation}
\label{eq:uniqueness-implication}
\setdef{j \in \bar{\mc E}}{\tau_j = \sigma_i, \, R_{ji} > 0} \neq \emptyset, \qquad \forall \, i \in \bar{\mc E}
\end{equation}
%Let $\bar{\mc G}:=(\mc V, \bar{\mc E})$. 

\ksmargin{show $v$, $j_2$, $j_3$ in Fig~\ref{fig:uniqueness}}
\begin{figure}[htb!]
\begin{center}				
\includegraphics[width=1.52in,angle=270]{../CDC2017/fig/uniqueness-illustration.pdf} 
\end{center}
\caption{Illustration of construction to prove uniqueness of solution to \eqref{z-linprog} by construction.}
\label{fig:uniqueness}
\end{figure}

Pick an arbitrary node $v \in \mc V$ such that $\bar{\mc E}_v^- \neq \emptyset$. Let $j_1 = \argmax_{i \in \mc E_v^-} z_i$ (ties are broken arbitrarily). Following \eqref{eq:uniqueness-implication}, let $j_2:=\argmax_{i \in \bar{\mc E}_{\sigma(j_1)}^-: \, R_{i j_1} > 0} \, z_i$, with ties broken arbitrarily. The definition of $j_2$, along \eqref{eq:uniqueness} implies that $z_{j_1} \leq z_{j_2}$.
%
%and the fact that $R_{ij} < 1$ for all $i, j \in \mc E$, implies that $b_{j_1} < b_{j_2}$. 
One can similarly find $j_3$ such that $z_{j_1} \leq z_{j_2} \leq z_{j_3}$. Following \eqref{eq:uniqueness-implication}, this process can be repeated at most $m \leq |\mc V|$ times, when 
\begin{equation}
\label{eq:b-inequalities}
0<z_{j_1} \leq \ldots \leq z_{j_m}
\end{equation}
$\sigma_{j_m}=\tau_{j_k}$ for some $k \in \until{m}$: see Figure~\ref{fig:uniqueness} for illustration. The definition of $j_k$ along with \eqref{eq:uniqueness-implication} then implies that $z_{j_m} \geq z_{j_k}$, which, in light of \eqref{eq:b-inequalities}, can be true only if $z_{j_k} = \ldots z_{j_m}$. However, this implies that $R_{j_\ell j_{\ell+1}}=1$ for all $\ell \in \{k, \ldots,m-1\}$ and $R_{j_m j_1}=1$, i.e., the sub-network consisting of links $j_k, \ldots, j_m$ is disconnected from the rest of the network. In this case, \eqref{eq:uniqueness} holds true independently for this sub-network. However, this leads to a contradiction due to \eqref{eq:b-inequalities}. Therefore, $\bar{\mc E}=\emptyset$, and hence there does not exist $z \neq 0$ satisfying \eqref{eq:uniqueness}.
